# Supplementary material for: Application of pretrained universal machine-learning interatomic potential for physicochemical simulation of liquid electrolytes in Li-ion battery
Source: arXiv:2501.05211 ancillary file (2025-01-09)
Supplement: Supplementary file 1 [file Supporting_Information.pdf]

## Supporting Information

# Application of pretrained universal machine-learning interatomic potential for physicochemical simulation of liquid electrolytes in Li-ion battery

*Suyeon Ju,<sup>‡a</sup> Jinmu You,<sup>‡a</sup> Gijin Kim,<sup>a</sup> Yutack Park,<sup>a</sup> Hyungmin An,<sup>a</sup> and Seungwu Han<sup>\*ab</sup>*

<sup>a</sup> Department of Materials Science and Engineering and Research Institute of Advanced Materials, Seoul National University, Seoul 08826, Korea.

<sup>b</sup> Korea Institute for Advanced Study, Seoul 02455, Korea.

<sup>‡</sup>S.J. and J.Y. equally contributed to this work

\*Corresponding author: hansw@snu.ac.kr

**Table S1.** IUPAC names, abbreviations, and formulas of solvents and salts used in this paper.

| IUPAC name                               | Abbreviation       | Formula        | Image                                                                                 |
|------------------------------------------|--------------------|----------------|---------------------------------------------------------------------------------------|
| Ethylene carbonate                       | EC                 | $C_3H_4O_3$    | 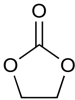   |
| Propylene carbonate                      | PC                 | $C_4H_6O_3$    | 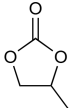   |
| Fluoroethylene carbonate                 | FEC                | $C_3H_3FO_3$   | 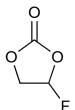   |
| Vinylene carbonate                       | VC                 | $C_3H_2O_3$    | 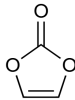   |
| <i>cis</i> -Difluoroethylene carbonate   | <i>cis</i> -DFEC   | $C_3H_2F_2O_3$ | 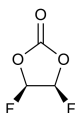 |
| <i>trans</i> -Difluoroethylene carbonate | <i>trans</i> -DFEC | $C_3H_2F_2O_3$ | 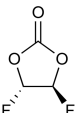 |
| Difluoroethylene carbonate               | DFEC               | $C_3H_2F_2O_3$ | 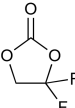 |
| $\gamma$ -Butyrolactone                  | GBL                | $C_4H_6O_2$    | 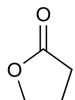 |
| Dimethyl carbonate                       | DMC                | $C_3H_6O_3$    | 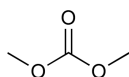 |
| Ethyl methyl carbonate                   | EMC                | $C_4H_8O_3$    | 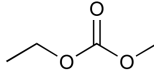 |

**Table S1.** (continued)

| IUPAC name                            | Abbreviation      | Formula           | Image                                                                                 |
|---------------------------------------|-------------------|-------------------|---------------------------------------------------------------------------------------|
| Diethyl carbonate                     | DEC               | $C_5H_{10}O_3$    | 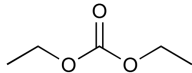   |
| Fluoromethyl methyl carbonate         | MFDMC             | $C_3H_5O_3F$      | 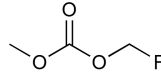   |
| Bis(fluoromethyl) carbonate           | DFDMC             | $C_3H_4O_3F_2$    | 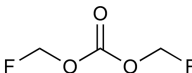   |
| Difluoromethyl fluoromethyl carbonate | TFDMC             | $C_3H_3O_3F_3$    | 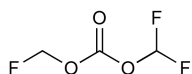   |
| 1,2-Dimethoxyethane                   | DME               | $C_4H_{10}O_2$    | 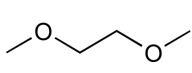   |
| 1,2-Diethoxyethane                    | DEE               | $C_6H_{14}O_2$    | 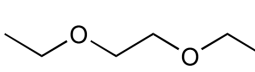  |
| Ethyl acetate                         | EA                | $C_4H_8O_2$       | 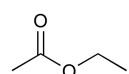 |
| Fluoroethyl acetate                   | FEA               | $C_4H_7O_2F$      | 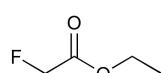 |
| Ethyl 2-fluoroacetate                 | EFA               | $C_4H_7O_2F$      | 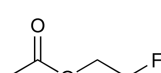 |
| Ethyl propionate                      | EP                | $C_5H_{10}O_2$    | 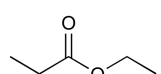 |
| Lithium hexafluorophosphate           | LiPF <sub>6</sub> | LiPF <sub>6</sub> | 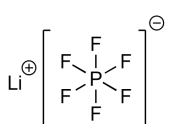 |
| Lithium bis(fluorosulfonyl)imide      | LiFSI             | $LiC_2NO_4F_6S_2$ | 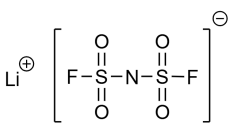 |

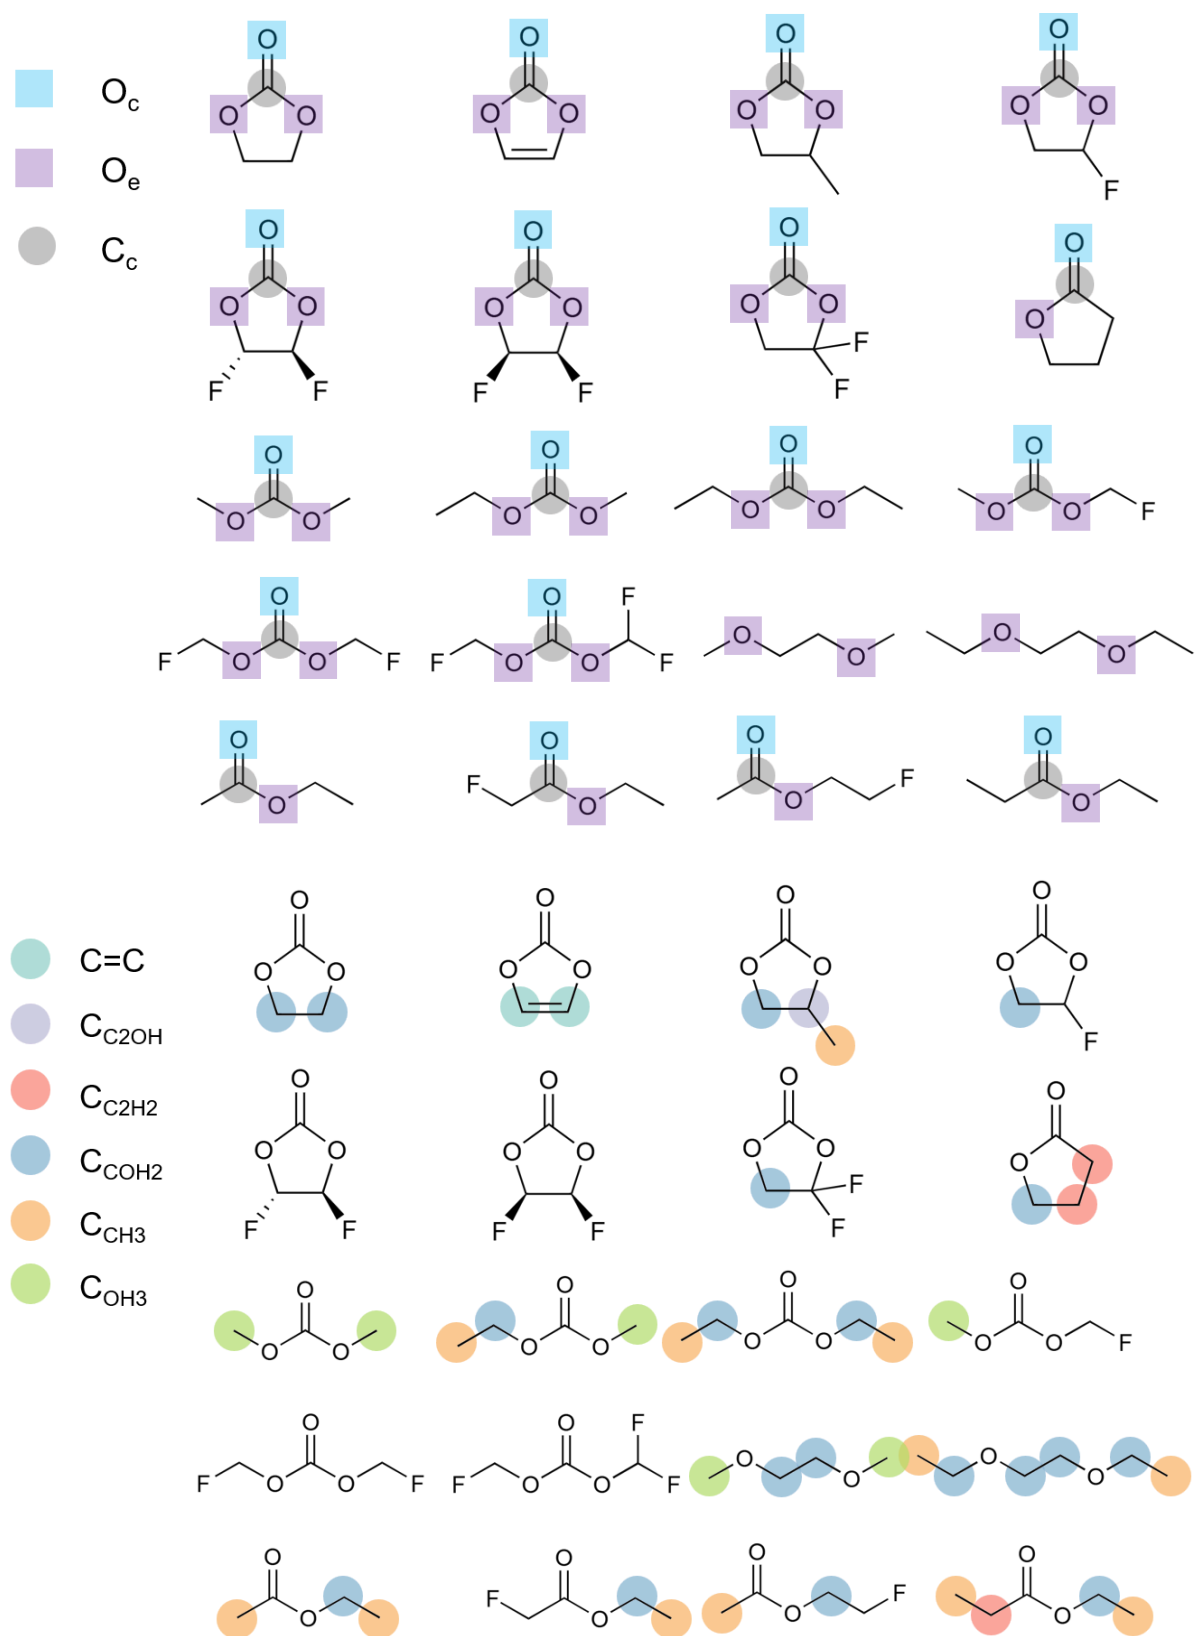

**Figure S1.** Classification of atom types in each solvent molecule.

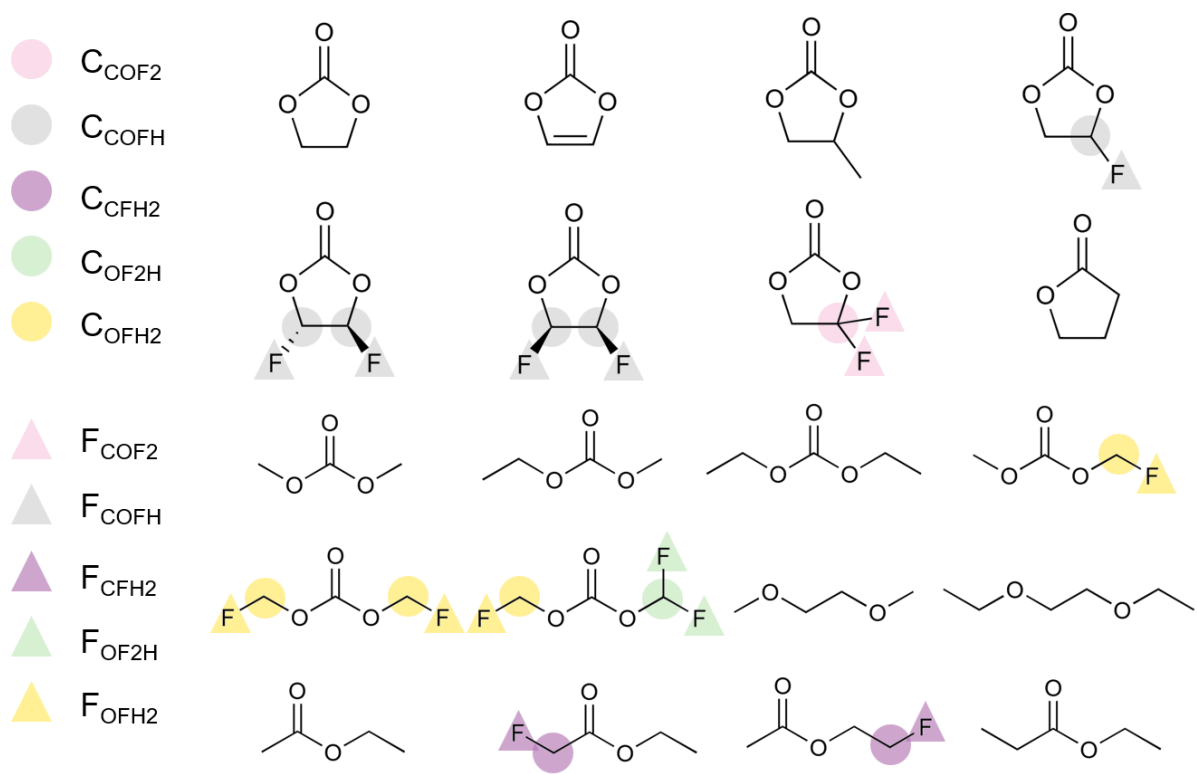

**Figure S1.** (continued)

### Procedure to classify atom types

The oxygen atoms are divided into carbonyl ( $O_c$ ) and ethereal ( $O_e$ ) oxygens. Carbon atoms are categorized based on their bonding environments; for example, the  $C_{COFH}$  represents a carbon atom bonded to one carbon, one oxygen, one fluorine, and one hydrogen atom. Double-bonded carbons in VC are classified separately. For fluorine atoms, it is difficult to differentiate their environments using only information about their neighbors. Therefore, we use the neighbors of the carbon atom bonded to the fluorine atom to classify different fluorine atom types. This approach provides unique fluorine atom types, as only one carbon atom is bonded to all fluorine atoms in our 20 solvent systems. For example,  $F_{COFH}$  represents a fluorine atom bonded to a carbon atom, where the carbon atom has neighbors consisting of one carbon, one oxygen, one fluorine, and one hydrogen.

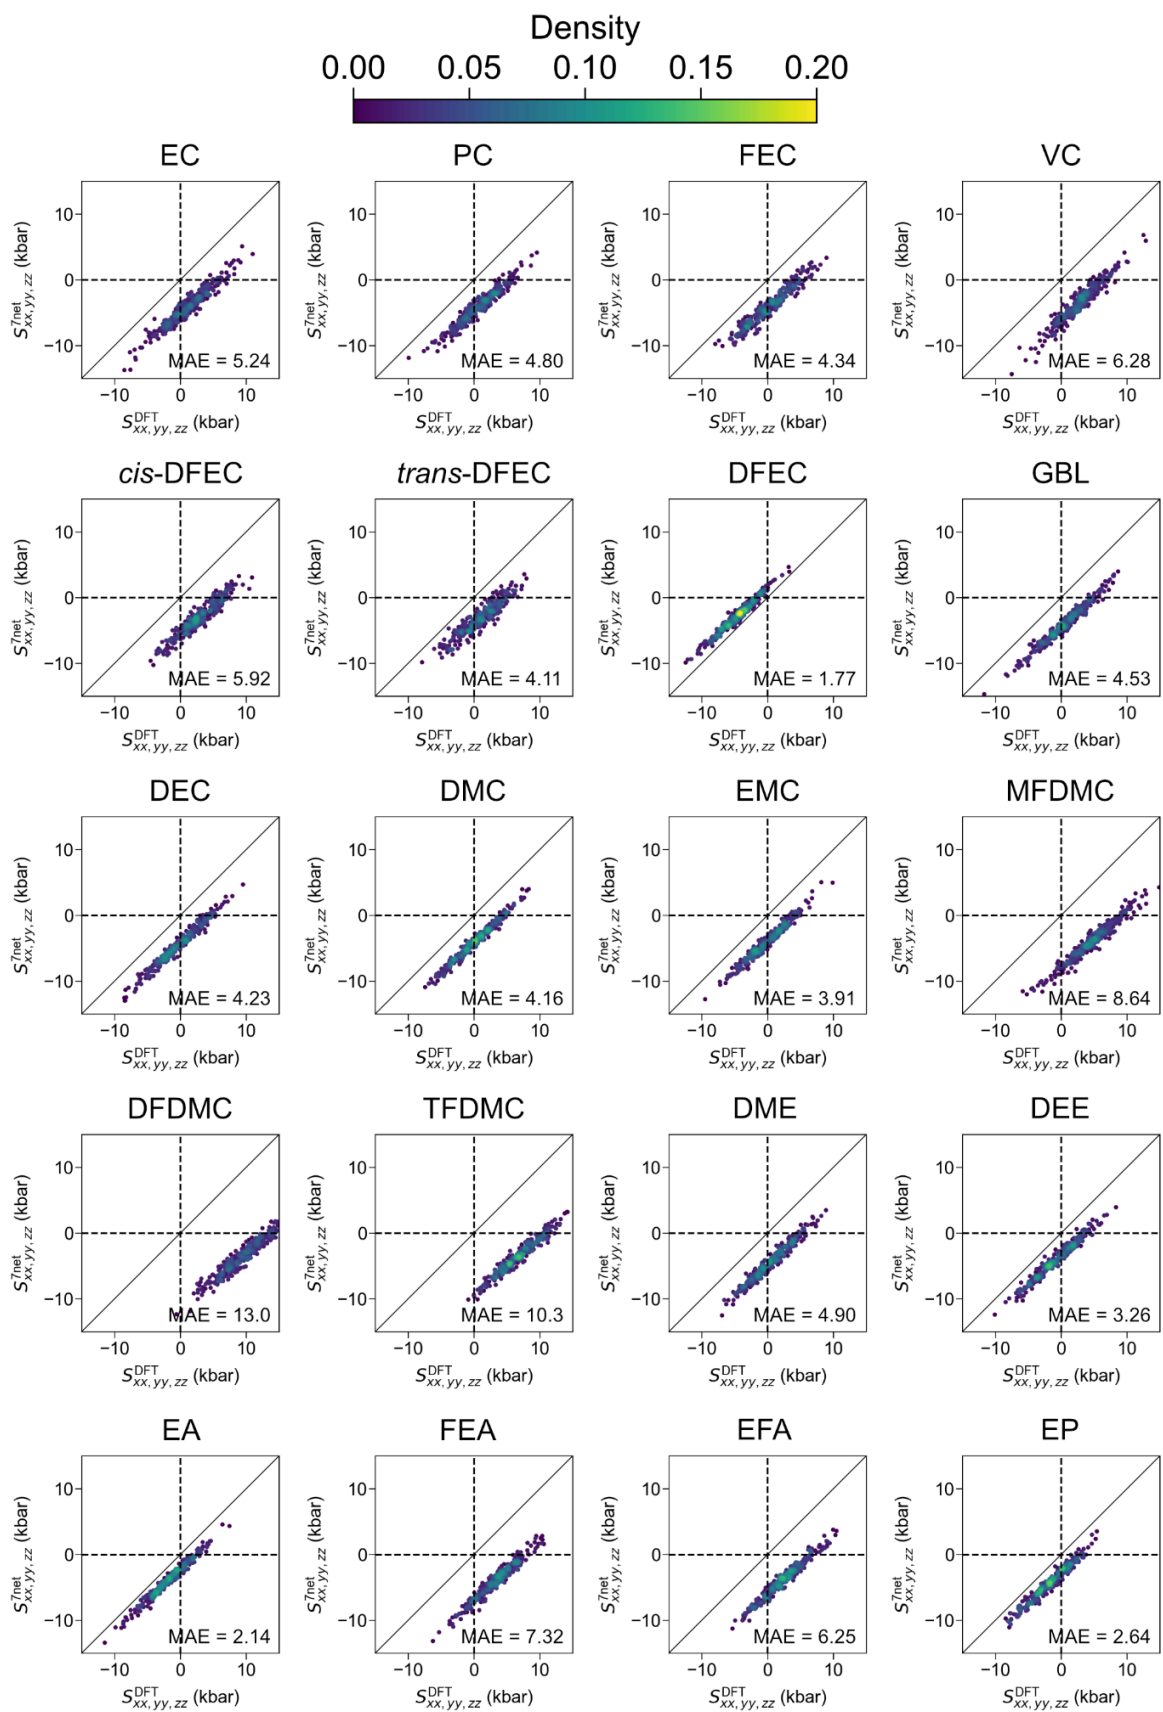

**Figure S2.** Normal stress parity plots for pure solvents calculated with SevenNet.

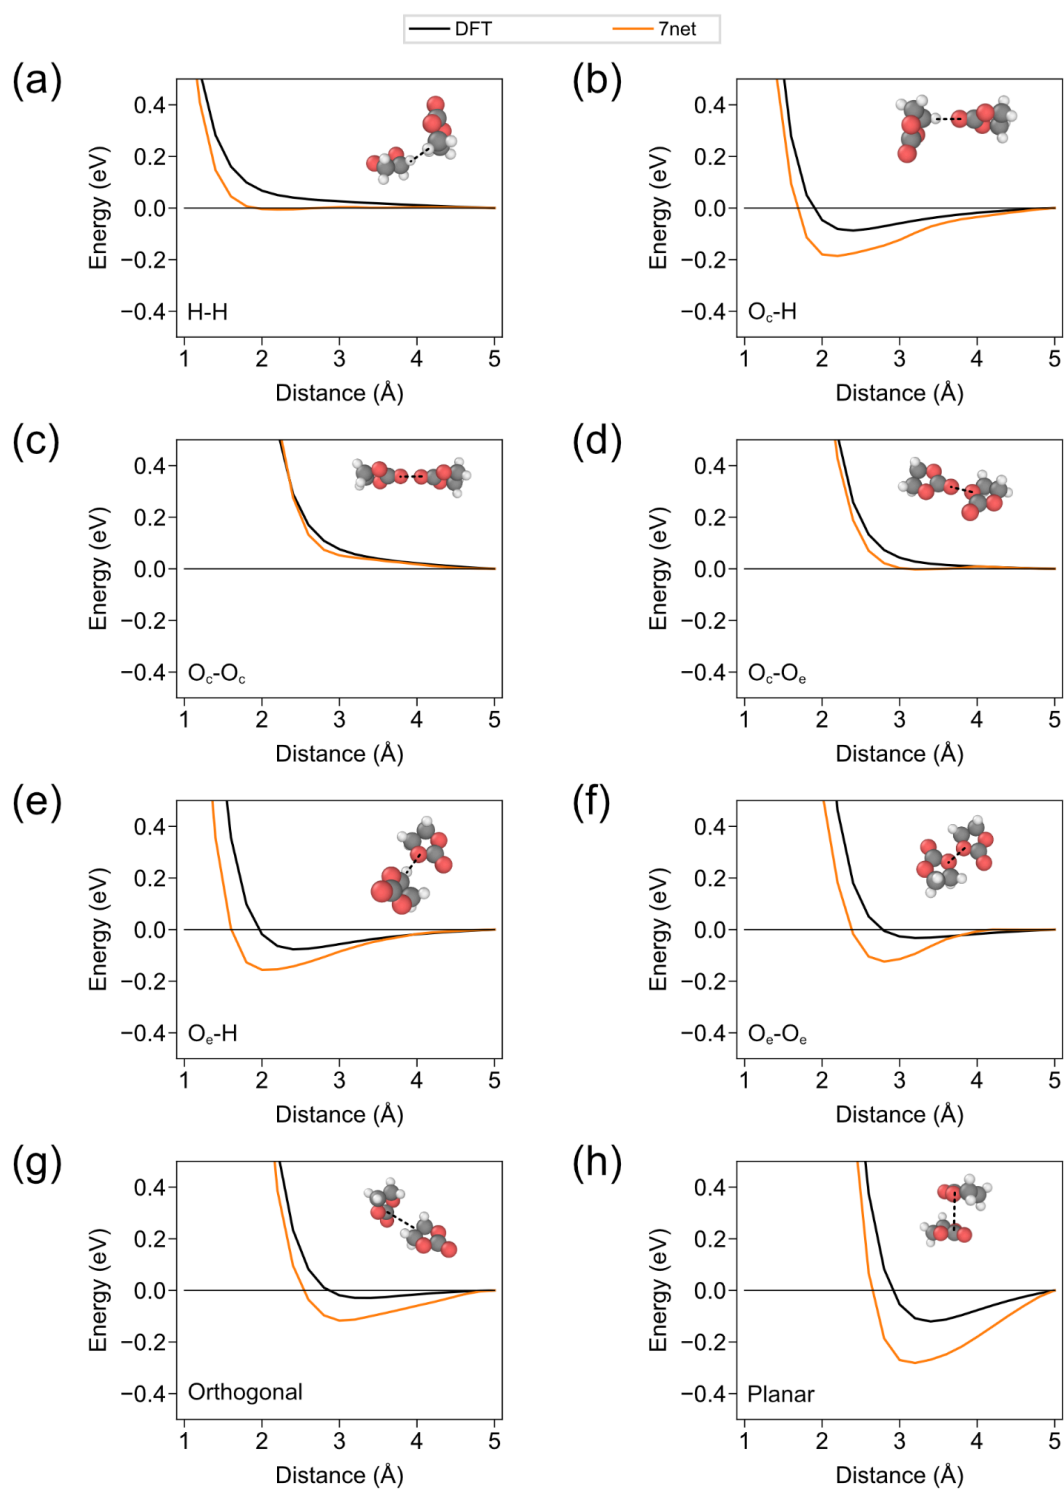

**Figure S3.** Potential energy curve of EC dimer obtained from SevenNet compared to DFT values according to the distance of (a) H-H, (b)  $O_c$ -H, (c)  $O_c$ - $O_c$ , (d)  $O_c$ - $O_e$ , (e)  $O_e$ -H, (f)  $O_e$ - $O_e$ , (g) orthogonal orientation of dimer ( $C_c$  and positional average of 4 hydrogen), and (h) planar orientation of dimer ( $C_c$  and  $C_c$ ).

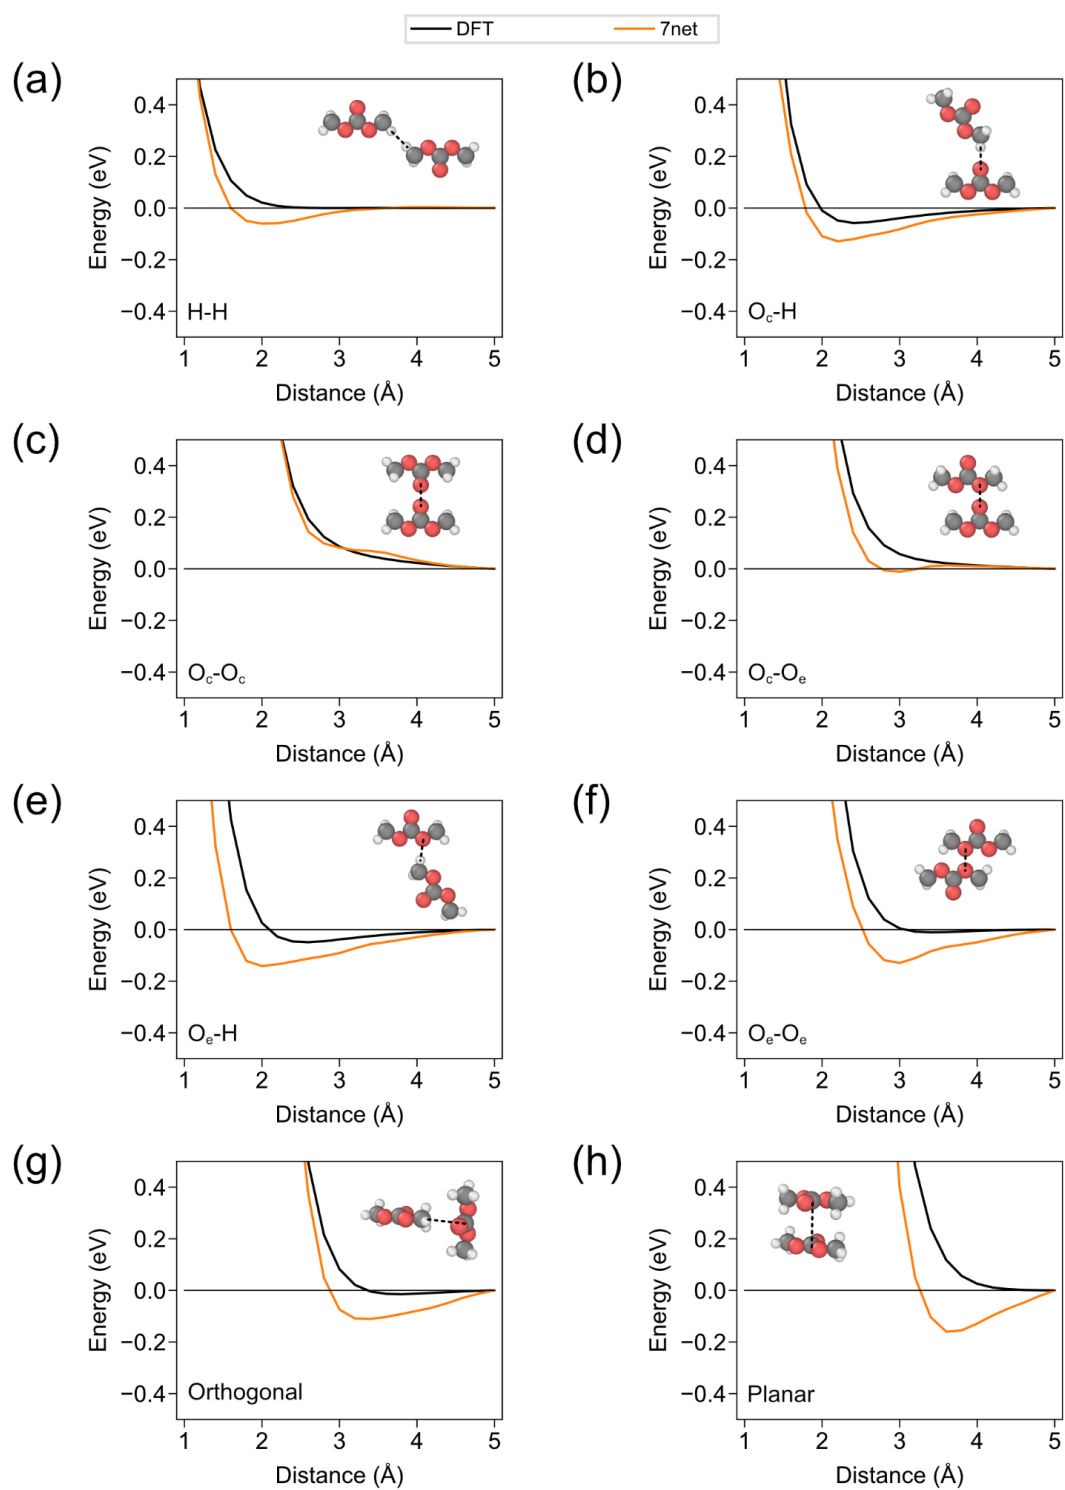

**Figure S4.** Potential energy curve of DMC dimer obtained from SevenNet compared to DFT values according to the distance of (a) H-H, (b)  $O_c$ -H, (c)  $O_c$ - $O_c$ , (d)  $O_c$ - $O_e$ , (e)  $O_e$ -H, (f)  $O_e$ - $O_e$ , (g) orthogonal orientation of dimer ( $C_c$  and positional average of 4 hydrogen), and (h) planar orientation of dimer ( $C_c$  and  $C_c$ ).

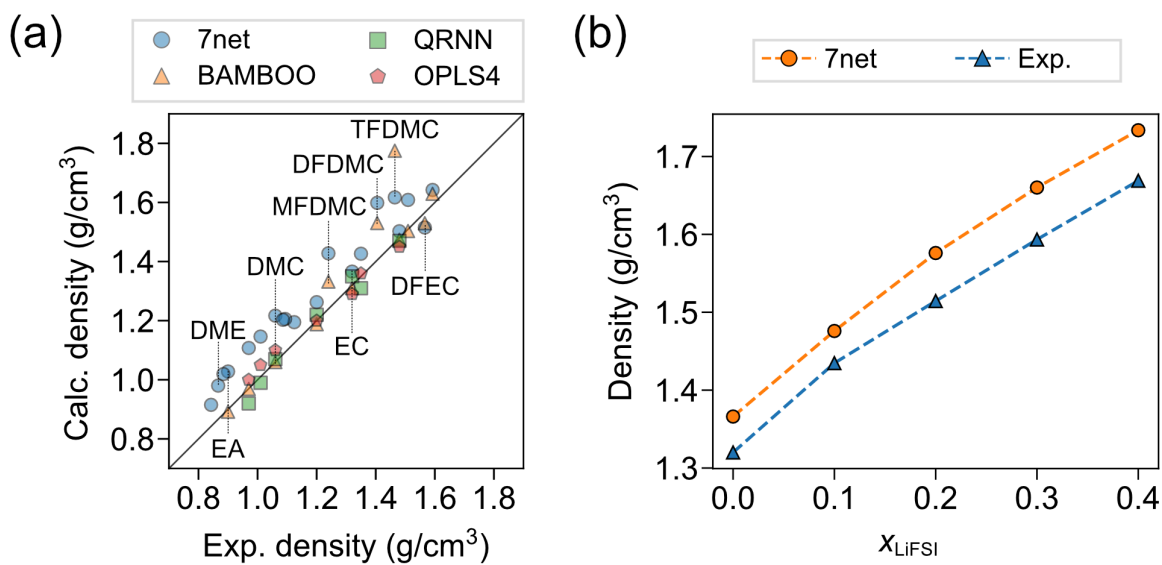

**Figure S5.** (a) Parity plot comparing pure solvent densities obtained using SevenNet (blue circles), BAMBOO (orange triangles), QRNN (green squares), and OPLS4 (red pentagons) method and experiments. See Table S5 for the actual values and errors. The MD simulations were conducted at 298 K, except for EC (313 K), FEC (313 K), DME (293 K), and DEE (293 K). (b) Density obtained by SevenNet compared to experimental values<sup>1,2</sup> with increasing LiFSI molar ratio in EC solvent system at 313 K.

### Analysis of Fig. S5b

The density of the EC/LiFSI electrolyte system shows that the calculated values using SevenNet qualitatively follow the experimental trend, systematically overestimating the experimental densities by 3–4% across the entire concentration range. Details in the initial structures are summarized in Table S9. It is worthy noting that  $x_{\text{LiFSI}} = 0.4$  corresponds to a concentration of 4.5 M, which is considered high for liquid electrolytes. The calculated (experimental<sup>1,2</sup>) values are 1.367 (1.32), 1.472 (1.435), 1.572 (1.514), 1.649 (1.593), and 1.731 (1.669) g/cm³ for  $x_{\text{LiFSI}} = 0, 0.1, 0.2, 0.3$ , and 0.4, respectively.

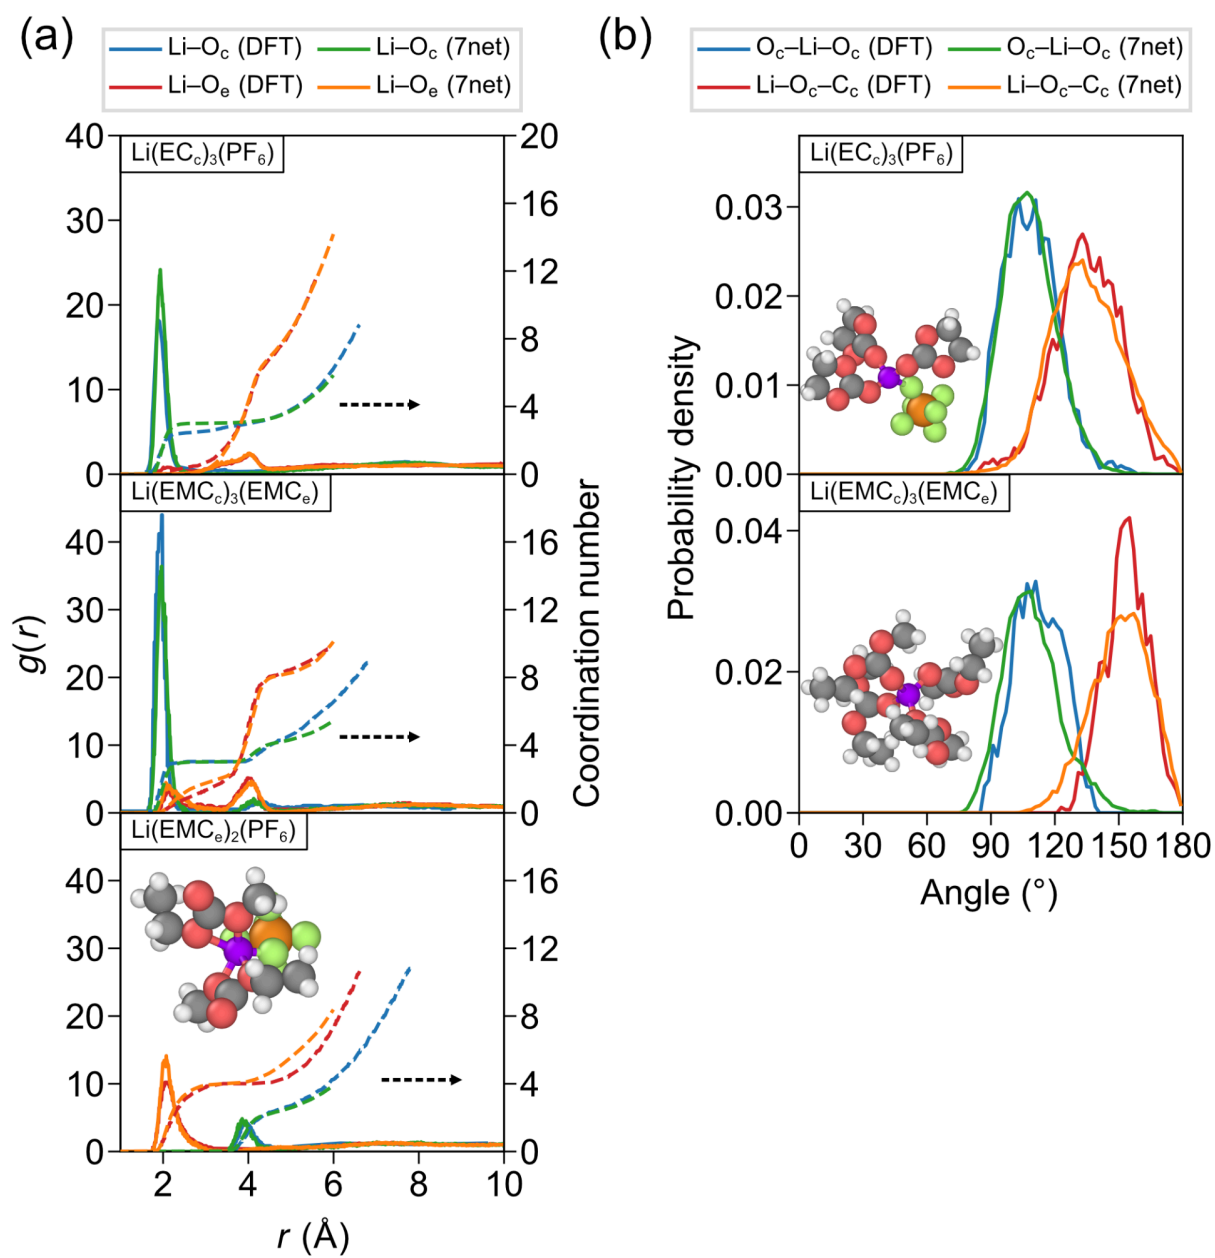

**Figure S6.** Solvation structures for  $\text{Li}(\text{EC}_c)_3(\text{PF}_6)$ ,  $\text{Li}(\text{EMCc})_3(\text{EMCc})$ , and  $\text{Li}(\text{EMCc})_2(\text{PF}_6)$  solvation types obtained by SevenNet, compared with DFT results.<sup>3</sup> (a) RDFs (solid lines) of Li-O<sub>c</sub> and Li-O<sub>e</sub> and their CNs (dashed lines) for each solvation type. (b) Angular distributions of O<sub>c</sub>-Li-O<sub>c</sub> and Li-O<sub>c</sub>-C<sub>c</sub> angles for each solvation type. Example structures of each solvation type are illustrated in the inset.

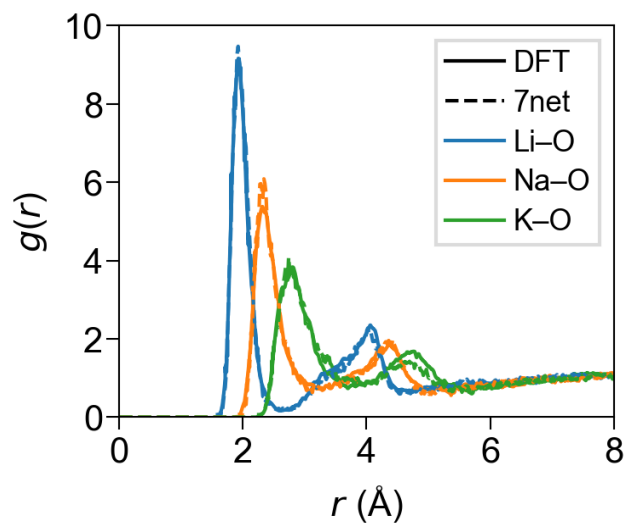

**Figure S7.** Radial distribution functions of Li, Na, and K cations between oxygens when solvated in EC molecules. Blue, orange, and green lines represent radial distribution functions from Li, Na, and K, respectively. The solid and dashed lines represent the results obtained from DFT calculations<sup>4</sup> and SevenNet, respectively.

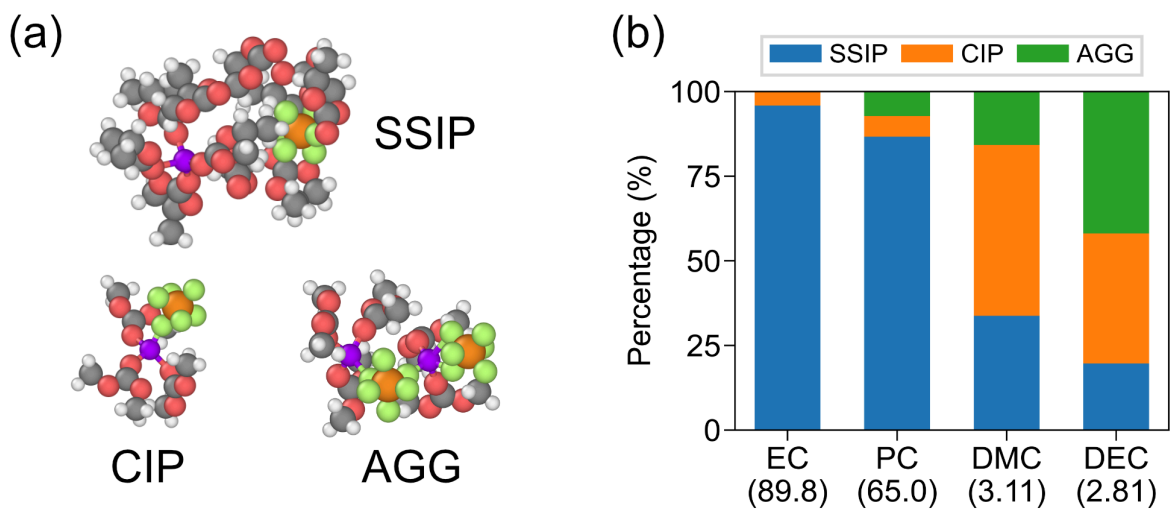

**Figure S8.** Variations in solvation environment among different types of solvents. (a) Representative SSIP, CIP, and AGG structures extracted from an MD trajectory of PC/1 M  $\text{LiPF}_6$  (SSIP) and DMC/1 M  $\text{LiPF}_6$  (CIP and AGG). (b) The average percentage of each Li solvation state of 1 M  $\text{LiPF}_6$  salt concentration in four carbonates. The values are averaged across five independent production runs. The dielectric constant at 298.15 K of each solvent is marked below the name of the solvent.<sup>1</sup>

### Procedure and analysis

Since the experimental density of EC/1 M  $\text{LiPF}_6$  is unavailable, all simulations are performed starting with NPT equilibration to ensure a fair comparison, following the density-obtaining scheme in the main manuscript to determine the average density. Initial structures for NPT equilibration were created similarly with pure solvent NPT simulation (see section 2.2 in the main manuscript and Table S7 for the detailed information of the structure). Starting with 1.0-ns equilibration with a 2-fs timestep and a hydrogen atomic mass of 3 a.u., 0.4 ns of additional NPT simulation with a 1-fs timestep using the original hydrogen mass of 1 a.u. was conducted to obtain the initial configuration for the production run. Snapshots were saved every 100 fs, and a snapshot with a density closest to the average value over the last 0.2 ns of the NPT MD snapshots is selected as the initial structure of the NVT MD simulation.

(Equilibrated densities of PC, DMC, and DEC compositions are shown in Table S8. Equilibrated density of EC/1 M LiPF<sub>6</sub> is 1.461±0.001 g/cm<sup>3</sup>). Note that the densities are overestimated using SevenNet, which is present consistently at a high salt concentration regime in the EC/LiFSI system (Fig. S5b). Subsequently, a 1-ns production run in the NVT ensemble is conducted for solvation analysis. The results are averaged from five independent simulations with different initial structures. The temperatures are set at 293 K, except for DMC (298 K) to match the experimental conditions. Snapshots are saved every 100 fs during a 1-ns production run, and the solvation states of Li ions are analyzed below and averaged over all Li ions and snapshots.

Li ions are classified into three solvation states: SSIP, CIP, and AGG (Fig. S8a). A Li ion is classified as SSIP if it has no counter anion in its first solvation shell. If it has only one counter anion in its first solvation shell with no other Li ions near the counter anion, it is designated as CIP. If the Li ion is part of a cluster with more than three ions, it is classified as AGG.

The distribution of Li solvation states in each solvent, along with their respective dielectric constants, is presented in Fig. S8b. SSIPs dominate the solvation state in cyclic carbonates, underscoring the strong dielectric shielding provided by these solvents. Conversely, in linear carbonates, fewer Li ions are fully solvated by the solvent and more portion of CIPs and AGGs are observed during simulation. The average CN of the PF<sub>6</sub><sup>-</sup> counterion around Li<sup>+</sup> is 0.04, 0.21, 0.72, and 1.01 in EC, PC, DMC, and DEC, respectively, reflecting distinct solvation behaviors between solvent types. The dominance of LiPF<sub>6</sub> ion pairs in solvents with low dielectric constants and their dissociation in high dielectric constant solvents has been demonstrated by infrared spectroscopy analysis,<sup>5</sup> further supporting the trends observed in our study. These results demonstrate that the pretrained potential effectively captures the dynamic variations in dielectric shielding between cyclic and linear solvents.

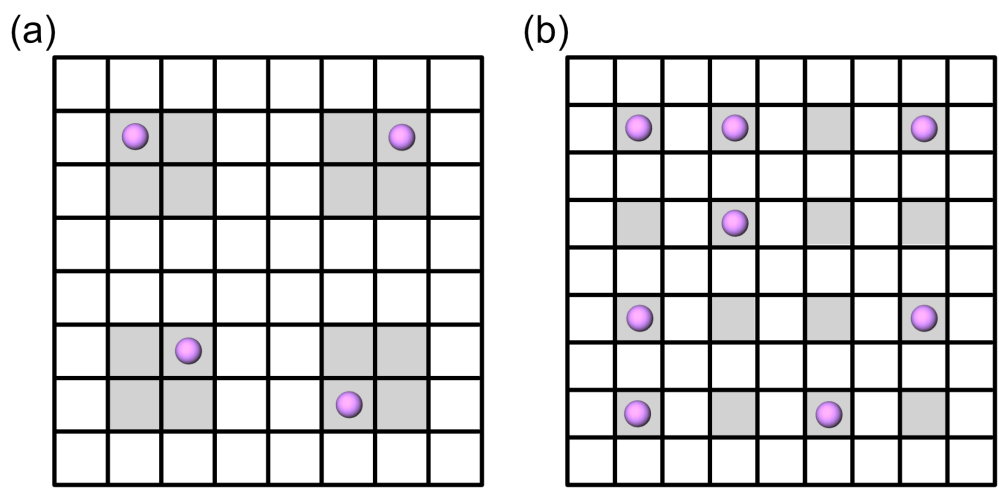

**Figure S9.** Schematic diagrams of placing Li ions within a cell with a top view along the x-axis. The shaded area indicates the possible location to place Li ions and the purple balls represent Li ions. (a) Method to place equal or less than 8 Li ions. The cubic box has dimensions of  $(1/8)a \times (1/8)a \times (1/8)a$ , where  $a$  is the length of the cell. (b) Method for placing up to 64 Li ions. The cubic box has dimensions of  $(1/9)a \times (1/9)a \times (1/9)a$ , where  $a$  is the length of the cell.

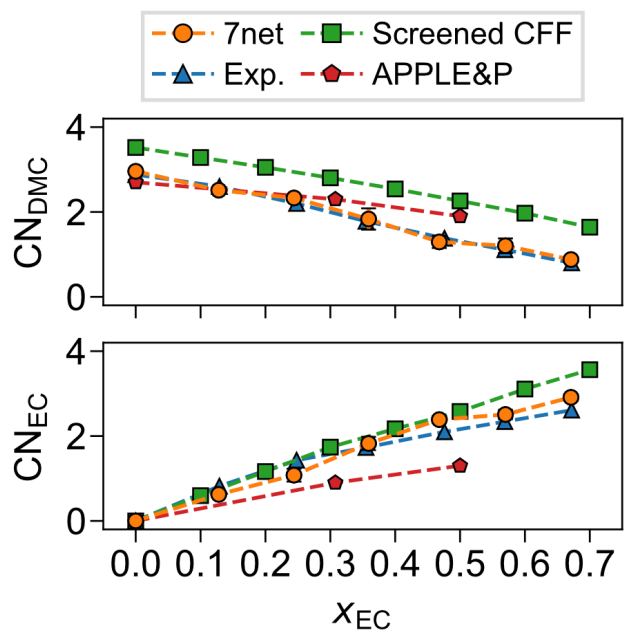

**Figure S10.** Average CNs of Li contributed by EC and DMC solvents in EC/DMC (1 mol/kg  $LiPF_6$ ) electrolyte at 298 K compared with experimental values<sup>6</sup> and results obtained from other force fields (Classical force fields with screened Coulomb interaction<sup>7</sup> and APPLE&P<sup>8</sup>).

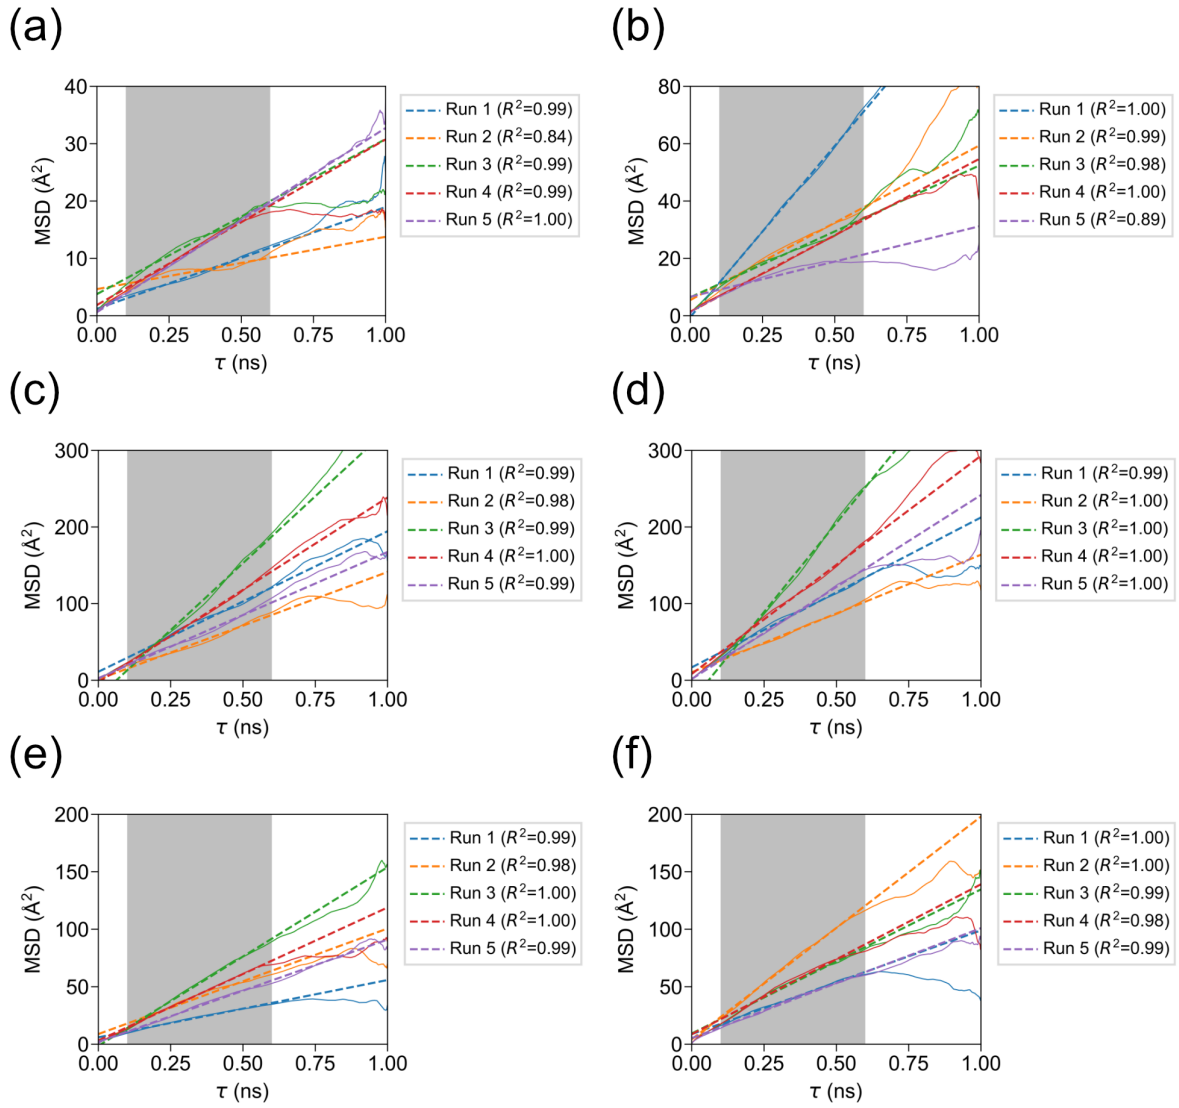

**Figure S11.** MSD- $\tau$  plots (solid lines) and the linear regression results (dashed lines). The  $R^2$  values from linear regression for each production run are shown in the legend. Gray boxes between 0.1 and 0.6 ns represent the linear regression region. Five independent runs are conducted for each system. (a) Results for Li ions and (b)  $\text{PF}_6^-$  anions in the PC/1 M  $\text{LiPF}_6$  electrolyte. (c) Results for Li ions and (d)  $\text{PF}_6^-$  anions in the DMC/1 M  $\text{LiPF}_6$  electrolyte. (e) Results for Li ions and (f)  $\text{PF}_6^-$  anions in the DEC/1 M  $\text{LiPF}_6$  electrolyte. All MD simulations are conducted at experimental densities by applying the NVT ensemble.

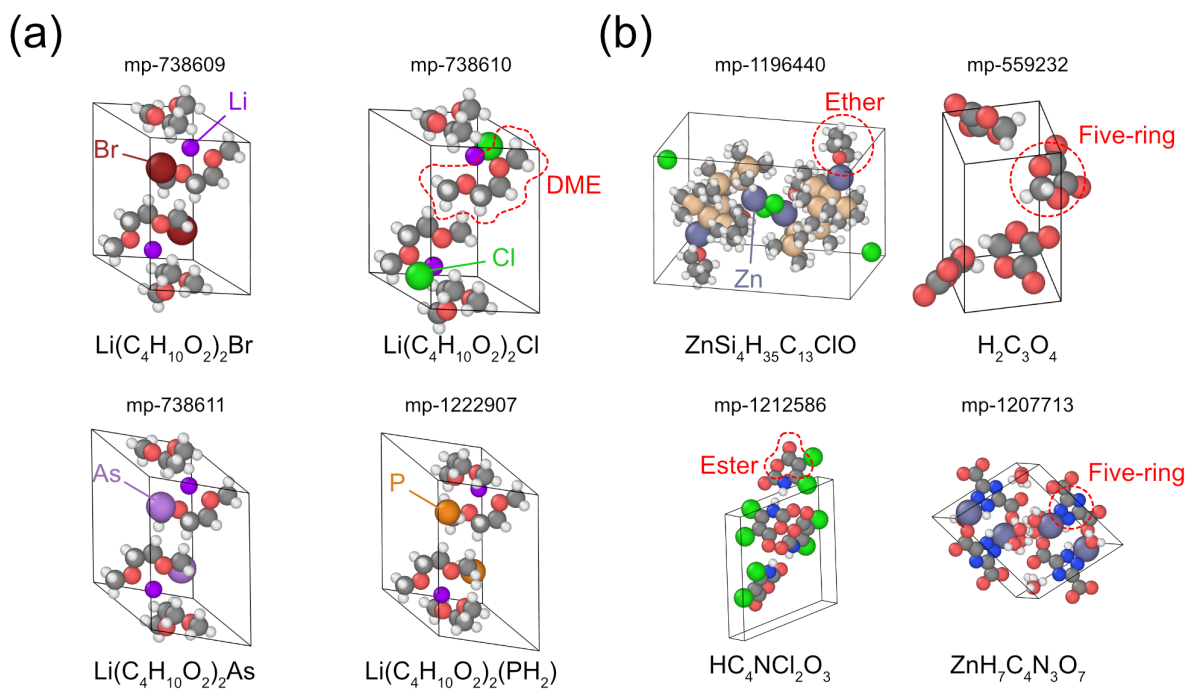

**Figure S12.** Similar or identical molecules with our solvent set in the training data. (a) All four structures in the training set that include DME molecules. (b) Representative similar molecules identified in the training set, featuring ether or ester groups, or containing five-membered ring structures.

### Procedure to find the molecular units

Since our solvents share common elements (O, C, and H), we filter out structures that lack at least one of these elements, narrowing the dataset of relaxation trajectories from 145 923 compounds to 22 909 snapshots. For further analysis, we use snapshots from the final ionic step of the relaxation trajectory for each compound, totaling 1892 snapshots. In these structures, all metal elements are removed, leaving only metalloids and nonmetals. Bonds are assigned between atoms if the interatomic distance is less than the sum of the covalent radii of each atom plus 0.2 Å.<sup>9</sup> This process segments a structure into clusters, each represented by its chemical formula. This enables us to identify molecules by their chemical formula from

all separated clusters and reveals that none of the solvents of interest are present in the training set, except for DME (Fig. S12a).

Although the exact molecules are absent from the training set, structurally similar molecules may be present. To investigate this, we perform a manual inspection of clusters with an atomic count similar to that of our solvent set. The range of the number of atoms is set with a margin of two. For instance, when investigating three-carbon molecules, clusters containing 6–14 atoms are inspected, as three-carbon solvents in our solvent set range from 8 atoms (VC) to 12 atoms (DMC). For four-, five-, and six-carbon molecules, clusters containing 10–18, 15–20, and 20–24 atoms are investigated, respectively. Structures containing ether and ester groups, as well as five-ring moieties similar to the ring substructure in EC, are found (Fig. S12b).



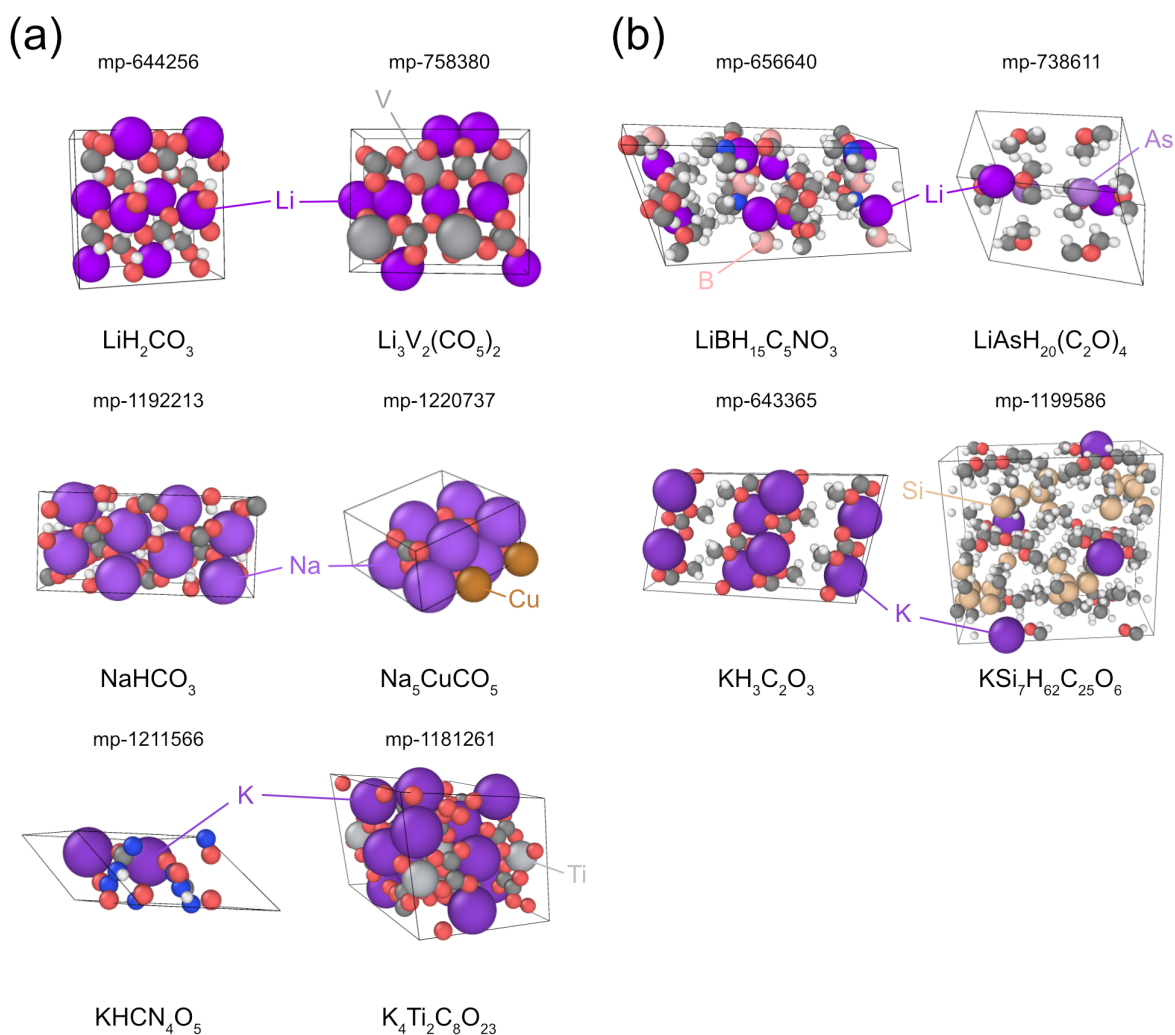

**Figure S14.** Structures from the training set containing (a) Li, Na, and K–O<sub>c</sub> bonds and (b) Li and K–O<sub>e</sub> bonds.

### Procedure to find the molecular units

After the procedure outlined in Fig. S13, structures with Li, Na, or K–O<sub>c</sub> bonds are filtered for Fig. S14a. Similarly, structures with Li, Na, or K–O<sub>e</sub> bonds are filtered for Fig. S14b, though no Na–O<sub>e</sub> bonds are identified.

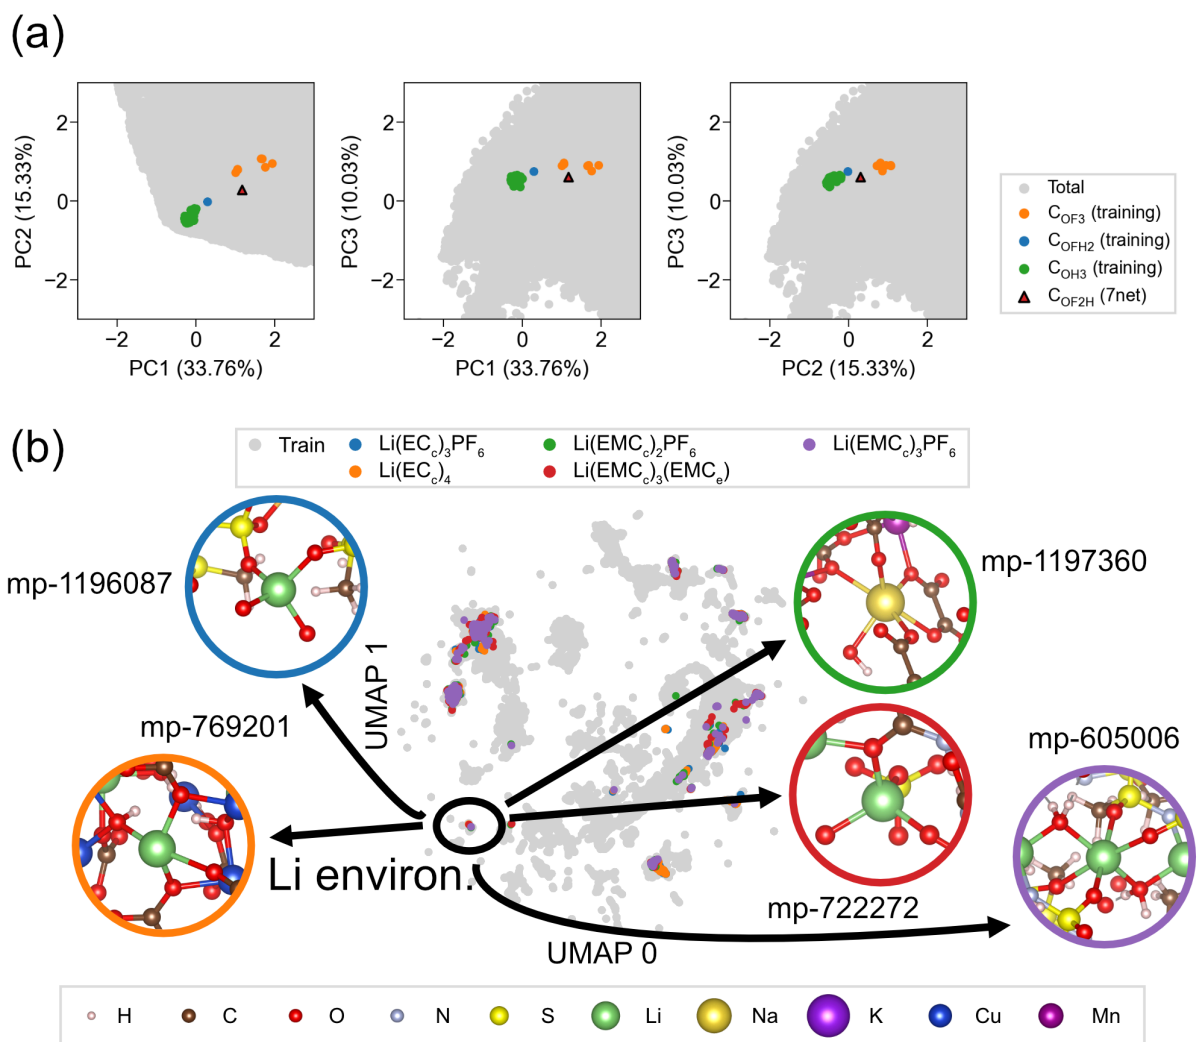

**Figure S15.** (a) The plot of latent vectors with principal component analysis (PCA). Circles represent PCA data points from the training set, while triangles represent PCA data points corresponding to the chemical moiety of C<sub>OF2H</sub> from TFDMC. The gray, orange, red, blue, and green colors represent the total training set, C<sub>OF3</sub>, C<sub>OF2H</sub>, C<sub>OFH2</sub>, and C<sub>OH3</sub> moieties, respectively. (b) UMAP analysis on the training set and test set. The test set consists of five solvation shell structures: Li(EC<sub>c</sub>)<sub>3</sub>PF<sub>6</sub> (blue), Li(EC<sub>c</sub>)<sub>4</sub> (orange), Li(EMC<sub>c</sub>)<sub>2</sub>PF<sub>6</sub> (green), Li(EMC<sub>c</sub>)<sub>3</sub>(EMC<sub>e</sub>) (red), and Li(EMC<sub>c</sub>)<sub>3</sub>PF<sub>6</sub> (purple). The gray circles represent the training set for SevenNet. The colored circles represent the structures in the training set that have the highest similarity to each test set structure. The Li environments are clustered in the black circle, and the O, C, and H environments are located outside.

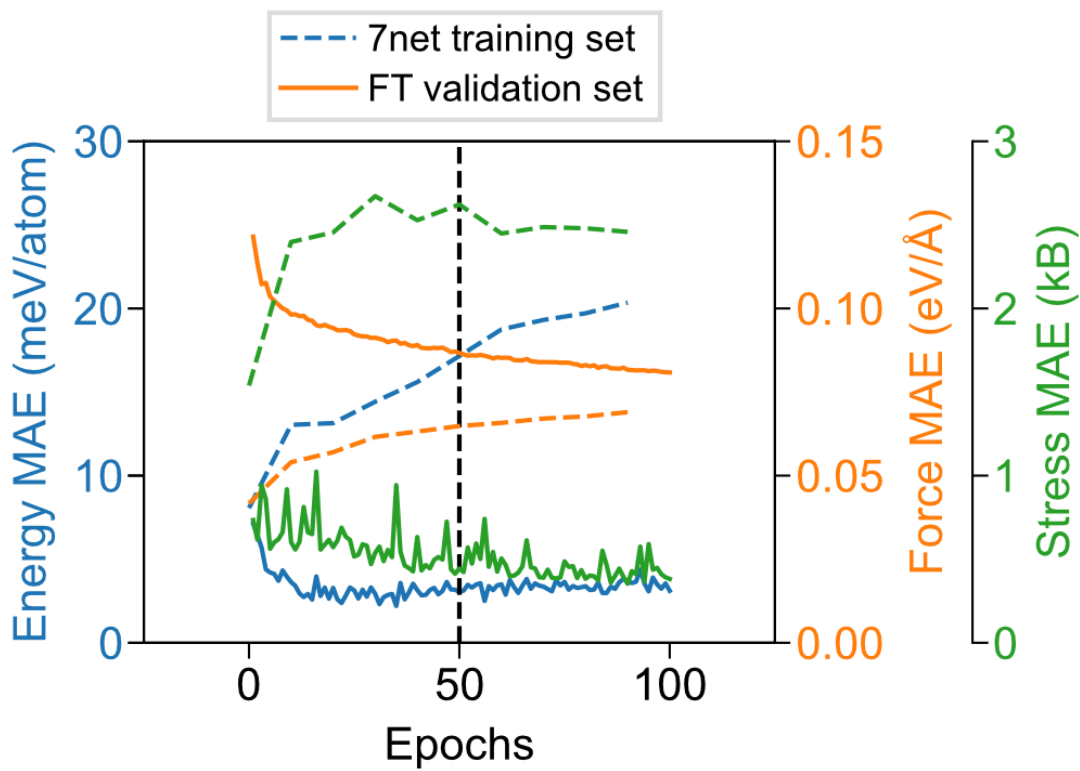

**Figure S16.** Training and validation results of fine-tuning procedure of SevenNet. The dashed lines indicate the MAEs of the fine-tuned potential with training epochs on the SevenNet training set filtered for the elements O, C, and H (19 072 structures). The solid lines demonstrate the learning curves of the validation set. Blue, orange, and green represent the energy, force, and stress MAEs, respectively.

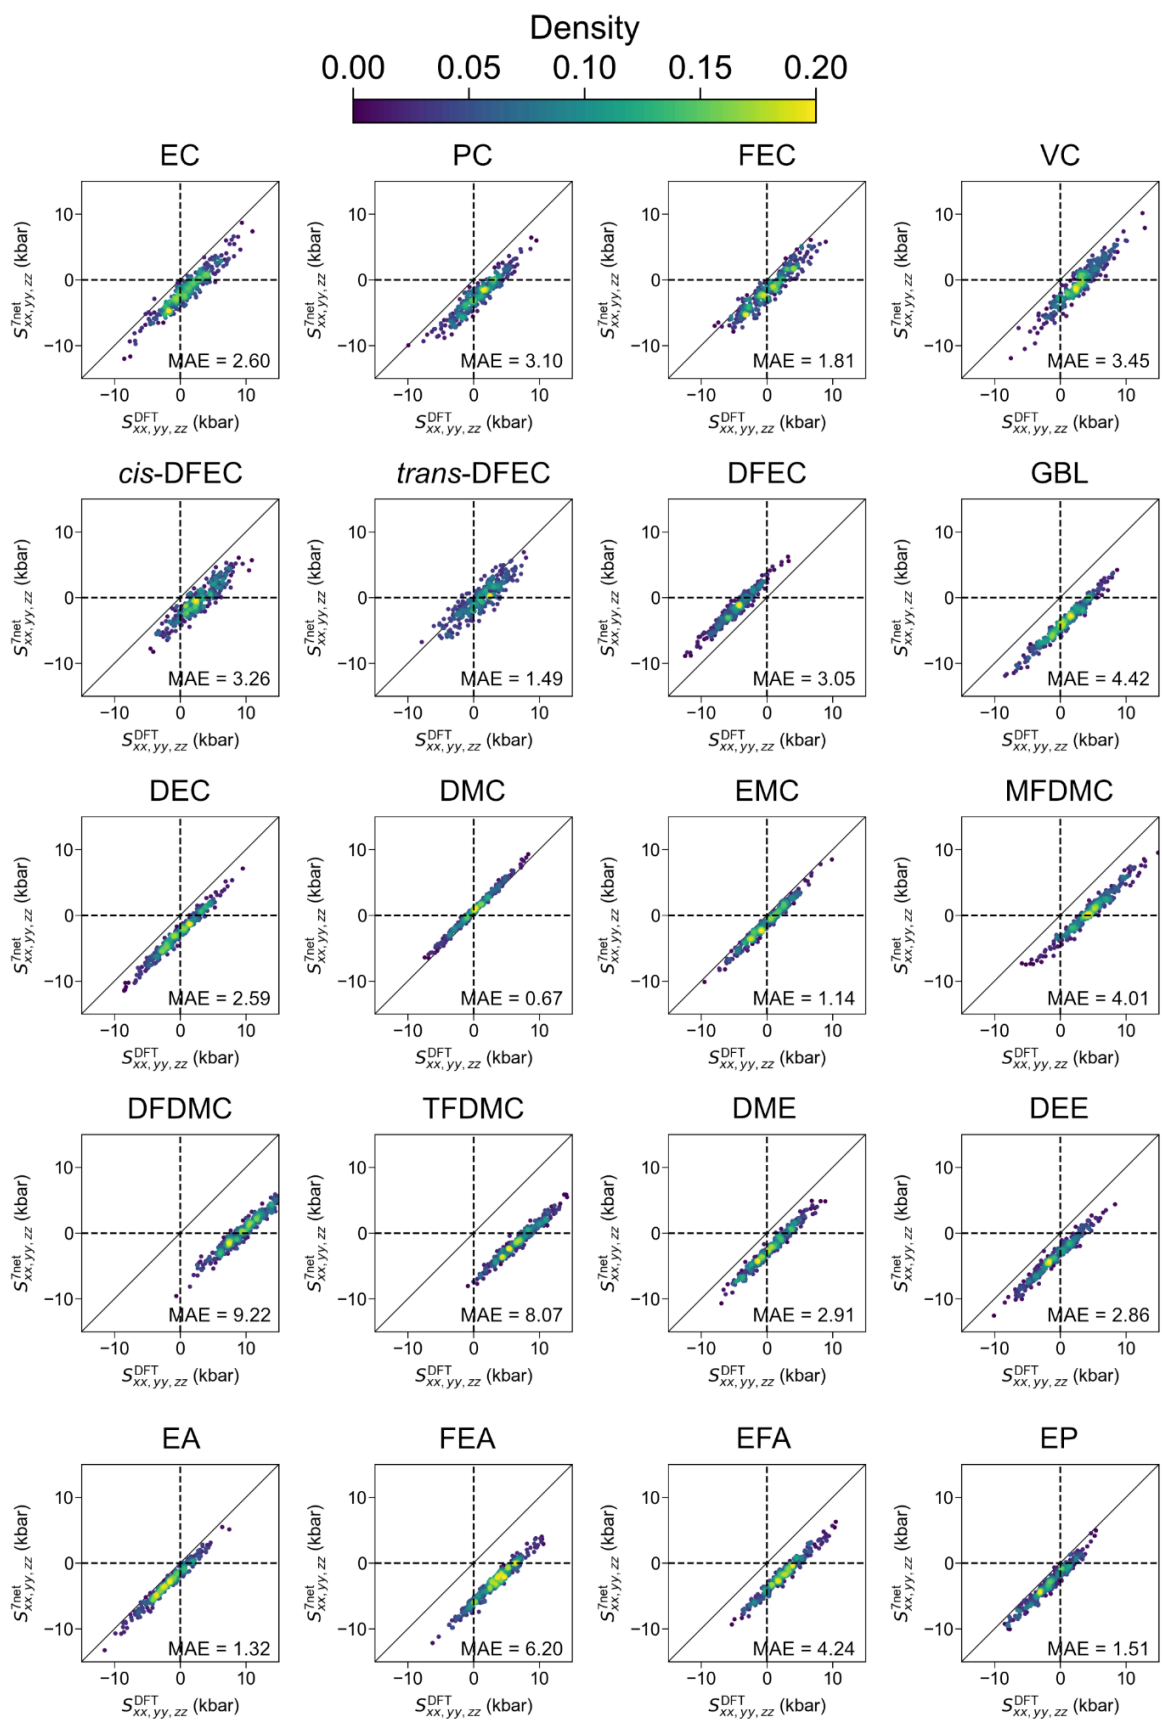

**Figure S17.** Normal stress parity plots for pure solvents calculated with SevenNet-FT.

**Table S2.** Details of initial cubic structures for density calculation of pure solvents.

| <b>Solvents</b>    | <b>Box length (Å)</b> | <b>Number of molecules</b>                  | <b>Number of atoms</b> |
|--------------------|-----------------------|---------------------------------------------|------------------------|
| EC                 | 23.40                 | EC (100)                                    | 1000                   |
| PC                 | 23.39                 | ( <i>S</i> )-PC (40) ( <i>R</i> )-PC (40)   | 1040                   |
| FEC                | 23.86                 | ( <i>S</i> )-FEC (50) ( <i>R</i> )-FEC (50) | 1000                   |
| VC                 | 24.46                 | VC (125)                                    | 1000                   |
| <i>cis</i> -DFEC   | 24.31                 | <i>cis</i> -DFEC (100)                      | 1000                   |
| <i>trans</i> -DFEC | 24.31                 | <i>trans</i> -DFEC (100)                    | 1000                   |
| DFEC               | 24.31                 | DFEC (100)                                  | 1000                   |
| GBL                | 22.65                 | GBL (80)                                    | 960                    |
| DEC                | 22.21                 | DEC (54)                                    | 972                    |
| DMC                | 22.34                 | DMC (80)                                    | 960                    |
| EMC                | 22.43                 | EMC (66)                                    | 975                    |
| MFDMC              | 22.74                 | MFDMC (80)                                  | 960                    |
| DFDMC              | 23.14                 | DFDMC (80)                                  | 960                    |
| TFDMC              | 23.51                 | TFDMC (80)                                  | 960                    |
| DME                | 21.82                 | DME (62)                                    | 992                    |
| DEE                | 21.82                 | DEE (45)                                    | 990                    |
| EA                 | 22.20                 | EA (70)                                     | 980                    |
| FEA                | 22.56                 | FEA (70)                                    | 980                    |
| EFA                | 22.56                 | EFA (70)                                    | 980                    |
| EP                 | 22.30                 | EP (59)                                     | 1003                   |

**Table S3.** Conformer ratios and schematic conformer images of linear carbonates.

| Solvents | Ratio of<br><i>cis-cis</i> :<br><i>cis-trans</i> :<br><i>trans-cis</i> | Image of <i>cis-cis</i>                                                             | Image of <i>cis-trans</i>                                                            | Image of <i>trans-cis</i>                                                             |
|----------|------------------------------------------------------------------------|-------------------------------------------------------------------------------------|--------------------------------------------------------------------------------------|---------------------------------------------------------------------------------------|
| DEC      | 0.76:0.24                                                              | 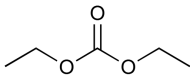   | 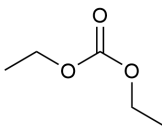   | -                                                                                     |
| DMC      | 0.76:0.24                                                              | 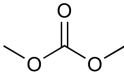   | 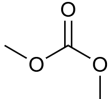   | -                                                                                     |
| EMC      | 0.65:0.22:0.12                                                         | 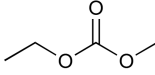   | 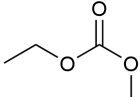   | 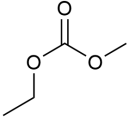   |
| MFDMC    | 0.89:0.11:0.00                                                         | 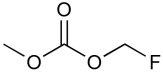  | 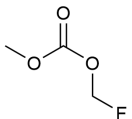  | 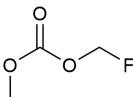  |
| DFDMC    | 0.66:0.34                                                              | 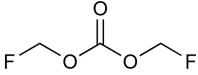 | 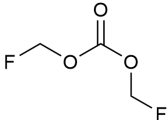 | -                                                                                     |
| TFDMC    | 0.47:0.13:0.40                                                         | 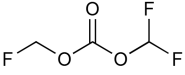 | 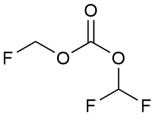 | 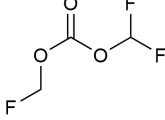 |

**Table S4.** Conformer ratios and scheschematic conformer images of esters.

|     | Ratio of<br><i>syn:anti</i> | Image of <i>syn</i>                                                               | Image of <i>anti</i>                                                                 |
|-----|-----------------------------|-----------------------------------------------------------------------------------|--------------------------------------------------------------------------------------|
| EA  | 0.99:0.01                   | 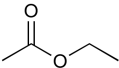 | 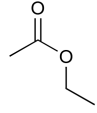  |
| FEA | 1.00:0.00                   | 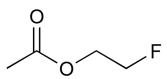 | 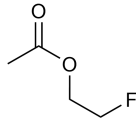  |
| EFA | 0.89:0.11                   | 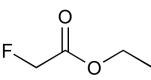 | 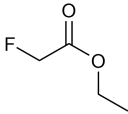  |
| EP  | 0.99:0.01                   | 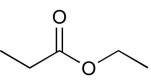 | 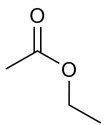 |

**Table S5.** Calculated and experimental density values of pure solvents with their errors with respect to experimental densities. ‘Cyclic’ and ‘Linear’ represents cyclic carbonates and linear carbonates, respectively. GBL is an ester molecule with a cyclic structure. Ethers and other esters have linear structure.

| Solvents           | Type   | Temperature (K) | Calculated density (g/cm <sup>3</sup> ) | Experimental density (g/cm <sup>3</sup> ) | Error (%) |
|--------------------|--------|-----------------|-----------------------------------------|-------------------------------------------|-----------|
| EC                 | Cyclic | 313             | 1.3661                                  | 1.32 <sup>1</sup>                         | 3.6       |
| PC                 | Cyclic | 298             | 1.2627                                  | 1.2 <sup>10</sup>                         | 5.5       |
| FEC                | Cyclic | 313             | 1.5027                                  | 1.48 <sup>11</sup>                        | 1.6       |
| VC                 | Cyclic | 298             | 1.4266                                  | 1.35 <sup>10</sup>                        | 4.2       |
| <i>cis</i> -DFEC   | Cyclic | 298             | 1.6425                                  | 1.5924 <sup>12</sup>                      | 3.5       |
| <i>trans</i> -DFEC | Cyclic | 298             | 1.6087                                  | 1.5093 <sup>12</sup>                      | 6.0       |
| DFEC               | Cyclic | 298             | 1.5153                                  | 1.5661 <sup>12</sup>                      | -3.3      |
| DEC                | Linear | 298             | 1.1077                                  | 0.97 <sup>1</sup>                         | 13.8      |
| DMC                | Linear | 298             | 1.2170                                  | 1.06 <sup>1</sup>                         | 14.5      |
| EMC                | Linear | 298             | 1.1463                                  | 1.01 <sup>1</sup>                         | 13.8      |
| MFDMC              | Linear | 298             | 1.4279                                  | 1.2397 <sup>12</sup>                      | 14.0      |
| DFDMC              | Linear | 298             | 1.5988                                  | 1.4050 <sup>12</sup>                      | 13.5      |
| TFDMC              | Linear | 298             | 1.6173                                  | 1.4645 <sup>12</sup>                      | 10.4      |
| DME                | Ether  | 293             | 0.9803                                  | 0.8665 <sup>13</sup>                      | 13.2      |
| DEE                | Ether  | 293             | 0.9153                                  | 0.8425 <sup>14</sup>                      | 8.2       |
| GBL                | Ester  | 298             | 1.1950                                  | 1.1239 <sup>15</sup>                      | 5.6       |
| EA                 | Ester  | 298             | 1.0281                                  | 0.9 <sup>16</sup>                         | 14.3      |
| FEA                | Ester  | 298             | 1.2058                                  | 1.0932 <sup>12</sup>                      | 10.7      |
| EFA                | Ester  | 298             | 1.2031                                  | 1.0858 <sup>12</sup>                      | 10.4      |
| EP                 | Ester  | 298             | 1.0194                                  | 0.8843 <sup>17</sup>                      | 15.2      |

**Table S6.** Details of initial cubic structures for NVT simulation of EC/DMC binary solvent system with 1 mol/kg LiPF<sub>6</sub> electrolyte systems.

| Solvents | Composition                                            | Box length (Å) | Number of molecules                                                        | Number of atoms |
|----------|--------------------------------------------------------|----------------|----------------------------------------------------------------------------|-----------------|
| EC/DMC   | $x_{\text{EC}} = 0.000/$<br>1 mol/kg LiPF <sub>6</sub> | 22.50          | EC (0), <i>cc</i> -DMC (70),<br><i>ct</i> -DMC (8), LiPF <sub>6</sub> (7)  | 992             |
| EC/DMC   | $x_{\text{EC}} = 0.128/$<br>1 mol/kg LiPF <sub>6</sub> | 22.29          | EC (10), <i>cc</i> -DMC (61),<br><i>ct</i> -DMC (7), LiPF <sub>6</sub> (7) | 972             |
| EC/DMC   | $x_{\text{EC}} = 0.248/$<br>1 mol/kg LiPF <sub>6</sub> | 22.09          | EC (19), <i>cc</i> -DMC (53),<br><i>ct</i> -DMC (6), LiPF <sub>6</sub> (7) | 954             |
| EC/DMC   | $x_{\text{EC}} = 0.359/$<br>1 mol/kg LiPF <sub>6</sub> | 21.90          | EC (28), <i>cc</i> -DMC (46),<br><i>ct</i> -DMC (4), LiPF <sub>6</sub> (7) | 936             |
| EC/DMC   | $x_{\text{EC}} = 0.468/$<br>1 mol/kg LiPF <sub>6</sub> | 21.85          | EC (37), <i>cc</i> -DMC (39),<br><i>ct</i> -DMC (3), LiPF <sub>6</sub> (7) | 930             |
| EC/DMC   | $x_{\text{EC}} = 0.570/$<br>1 mol/kg LiPF <sub>6</sub> | 21.67          | EC (45), <i>cc</i> -DMC (31),<br><i>ct</i> -DMC (3), LiPF <sub>6</sub> (7) | 914             |
| EC/DMC   | $x_{\text{EC}} = 0.671/$<br>1 mol/kg LiPF <sub>6</sub> | 21.55          | EC (53), <i>cc</i> -DMC (24),<br><i>ct</i> -DMC (2), LiPF <sub>6</sub> (7) | 898             |

**Table S7.** Details of initial cubic structures for four carbonate systems with 1 M LiPF<sub>6</sub> compositions.

| <b>Solvents</b> | <b>Simulation method</b>                   | <b>Box length (Å)</b> | <b>Number of molecules</b>                                        | <b>Number of atoms</b> |
|-----------------|--------------------------------------------|-----------------------|-------------------------------------------------------------------|------------------------|
| PC              | NVT with lattice from experimental volume  | 22.65                 | ( <i>R</i> )-PC (39), ( <i>S</i> )-PC (39), LiPF <sub>6</sub> (7) | 1070                   |
| DMC             | NVT with lattice from experimental volume  | 22.66                 | DMC (80), LiPF <sub>6</sub> (7)                                   | 1016                   |
| DEC             | NVT with lattice from experimental volume  | 22.68                 | DEC (56), LiPF <sub>6</sub> (7)                                   | 1064                   |
| EC              | NPT with lattice from van der Waals volume | 26.33                 | EC (100), LiPF <sub>6</sub> (7)                                   | 1056                   |
| PC              | NPT with lattice from van der Waals volume | 24.92                 | ( <i>R</i> )-PC (39), ( <i>S</i> )-PC (39), LiPF <sub>6</sub> (7) | 1070                   |
| DMC             | NPT with lattice from van der Waals volume | 24.93                 | DMC (80), LiPF <sub>6</sub> (7)                                   | 1016                   |
| DEC             | NPT with lattice from van der Waals volume | 24.95                 | DEC (56), LiPF <sub>6</sub> (7)                                   | 1064                   |

**Table S8.** Mean and standard deviation for density and diffusivity values of three carbonate systems with 1 M LiPF<sub>6</sub> compositions.

|                          | PC                                   |                    | DMC                                  |                     | DEC                                  |                    |
|--------------------------|--------------------------------------|--------------------|--------------------------------------|---------------------|--------------------------------------|--------------------|
|                          | $D_{Li}$                             | $D_{PF_6}$         | $D_{Li}$                             | $D_{PF_6}$          | $D_{Li}$                             | $D_{PF_6}$         |
|                          | $(10^{-6} \text{ cm}^2/\text{s})$    |                    | $(10^{-6} \text{ cm}^2/\text{s})$    |                     | $(10^{-6} \text{ cm}^2/\text{s})$    |                    |
| 7net-0 (NPT)             | 0.17±0.05                            | 0.28±0.11          | 1.01±0.27                            | 1.41±0.41           | 0.51±0.10                            | 0.85±0.29          |
|                          | 1.353±0.003 g/cm <sup>3</sup>        |                    | 1.308±0.004 g/cm <sup>3</sup>        |                     | 1.201±0.002 g/cm <sup>3</sup>        |                    |
| 7net-0 (NVT)             | 0.38±0.16                            | 0.99±0.59          | 3.60±1.39                            | 4.46±2.01           | 1.67±0.65                            | 2.12±0.69          |
|                          | 1.29 <sup>18</sup> g/cm <sup>3</sup> |                    | 1.18 <sup>19</sup> g/cm <sup>3</sup> |                     | 1.09 <sup>20</sup> g/cm <sup>3</sup> |                    |
| QRNN <sup>21</sup>       | 0.19 <sup>1</sup>                    | 0.54               | -                                    | -                   | 2.57                                 | 2.81               |
|                          | No information on the density        |                    |                                      |                     |                                      |                    |
| OPLS4 <sup>21</sup>      | 0.14                                 | 0.16               | -                                    | -                   | 0.25                                 | 0.31               |
|                          | No information on the density        |                    |                                      |                     |                                      |                    |
| TraPPE <sup>22</sup>     | 0.2 qq4                              | 0.59               | 1.11                                 | 1.11                | -                                    | -                  |
|                          | No information on the density        |                    |                                      |                     |                                      |                    |
| APPLE&P <sup>22,23</sup> | -                                    | -                  | 4.55                                 | 4.71                | -                                    | -                  |
|                          | -                                    |                    | 1.138 g/cm <sup>3</sup>              |                     | -                                    |                    |
| Experiment               | 0.69 <sup>24</sup>                   | 1.31 <sup>24</sup> | 3.745 <sup>25</sup>                  | 4.135 <sup>25</sup> | 2.27 <sup>24</sup>                   | 2.43 <sup>24</sup> |
|                          | 1.29 <sup>18</sup> g/cm <sup>3</sup> |                    | 1.18 <sup>19</sup> g/cm <sup>3</sup> |                     | 1.09 <sup>20</sup> g/cm <sup>3</sup> |                    |

**Table S9.** Details of initial cubic structures for different LiFSI concentrations in EC solvent.

| <b>Solvents</b> | <b>Composition</b>       | <b>Box length<br/>(Å)</b> | <b>Number of molecules</b> | <b>Number of atoms</b> |
|-----------------|--------------------------|---------------------------|----------------------------|------------------------|
| EC              | $x_{\text{LiFSI}} = 0.0$ | 23.40                     | EC (100)                   | 1000                   |
| EC              | $x_{\text{LiFSI}} = 0.1$ | 23.68                     | EC (90), LiFSI (10)        | 1000                   |
| EC              | $x_{\text{LiFSI}} = 0.2$ | 23.96                     | EC (80), LiFSI (20)        | 1000                   |
| EC              | $x_{\text{LiFSI}} = 0.3$ | 24.22                     | EC (70), LiFSI (30)        | 1000                   |
| EC              | $x_{\text{LiFSI}} = 0.4$ | 24.49                     | EC (60), LiFSI (40)        | 1000                   |

## References

- 1 K. Xu, *Chem. Rev.*, 2004, **104**, 4303–4418.
- 2 J. Neuhaus, E. von Harbou and H. Hasse, *J. Power Sources*, 2018, **394**, 148–159.
- 3 M. T. Ong, O. Verners, E. W. Draeger, A. C. T. van Duin, V. Lordi and J. E. Pask, *J. Phys. Chem. B*, 2015, **119**, 1535–1545.
- 4 T. A. Pham, K. E. Kweon, A. Samanta, V. Lordi and J. E. Pask, *J. Phys. Chem. C*, 2017, **121**, 21913–21920.
- 5 C. M. Burba and R. Frech, *J. Phys. Chem. B*, 2005, **109**, 15161–15164.
- 6 O. Borodin, M. Olguin, P. Ganesh, P. R. C. Kent, J. L. Allen and W. A. Henderson, *Phys. Chem. Chem. Phys.*, 2016, **18**, 164–175.
- 7 T. Kiyobayashi, S. Uchida, H. Ozaki and K. Kiyohara, *J. Chem. Phys.*, 2023, **159**, 074501.
- 8 B. Ravikumar, M. Mynam, S. Repaka and B. Rai, *J. Mol. Liq.*, 2021, **338**, 116613.
- 9 B. Cordero, V. Gómez, A. E. Platero-Prats, M. Revés, J. Echeverría, E. Cremades, F. Barragán and S. Alvarez, *Dalton Trans.*, 2008, 2832–2838.
- 10 R. Väli, A. Jänes and E. Lust, *J. Electrochem. Soc.*, 2016, **163**, A851–A857.
- 11 K. Hagiyaama, K. Suzuki, M. Ohtake, M. Shimada, N. Nanbu, M. Takehara, M. Ue and Y. Sasaki, *Chem. Lett.*, 2008, **37**, 210–211.
- 12 S. Gong, Y. Zhang, Z. Mu, Z. Pu, H. Wang, Z. Yu, M. Chen, T. Zheng, Z. Wang, L. Chen, X. Wu, S. Shi, W. Gao, W. Yan and L. Xiang, *arXiv*, 2024, preprint, arXiv:2404.07181, <https://arxiv.org/abs/2404.07181>.
- 13 P. Zheng, X. Meng, J. Wu and Z. Liu, *Int. J. Thermophys.*, 2008, **29**, 1244–1256.
- 14 M. Almasi, A. Hernández and J. Zarrini, *J. Chem. Eng. Data*, 2023, **68**, 1911–1920.
- 15 S.-K. Yang, S.-J. Peng, J.-H. Huang, L.-Q. Fan and F.-X. Yang, *J. Chem. Thermodyn.*, 2007, **39**, 773–780.

- 17 H. F. Costa, R. L. Gardas, I. Johnson, I. M. A. Fonseca and A. G. M. Ferreira, *J. Chem. Eng. Data*, 2009, **54**, 256–262.
- 18 M. Takeuchi, Y. Kameda, Y. Umebayashi, S. Ogawa, T. Sonoda, S. Ishiguro, M. Fujita and M. Sano, *J. Mol. Liq.*, 2009, **148**, 99–108.
- 19 SigmaAldrich, <https://www.sigmaaldrich.com/KR/ko/product/aldrich/746754> (accessed August 2024).
- 20 SigmaAldrich, <https://www.sigmaaldrich.com/KR/ko/product/aldrich/746770> (accessed August 2024).
- 21 S. Dajnowicz, G. Agarwal, J. M. Stevenson, L. D. Jacobson, F. Ramezanghorbani, K. Leswing, R. A. Friesner, M. D. Halls and R. Abel, *J. Phys. Chem. B*, 2022, **126**, 6271–6280.
- 22 Z. Luo, S. A. Burrows, S. K. Smoukov, X. Fan and E. S. Boek, *J. Phys. Chem. B*, 2023, **127**, 2224–2236.
- 23 O. Borodin and G. D. Smith, *J. Phys. Chem. B*, 2009, **113**, 1763–1776.
- 24 K. Hayamizu, *J. Chem. Eng. Data*, 2012, **57**, 2012–2017.
- 25 S. Miyoshi, H. Nagano, T. Fukuda, T. Kurihara, M. Watanabe, S. Ida and T. Ishihara, *J. Electrochem. Soc.*, 2016, **163**, A1206–A1213.
